# Supplementary material for: Towards FAIR protocols and workflows: The OpenPREDICT case study
Source: arXiv:1911.09531 source file (2019-11-20)
Supplement: Supplementary file 2 [file cs-43016-Appendix_2__OpenPREDICT_feature_generation_and_model_evaluation.pdf]

**Appendix 2: OpenPREDICT feature generation and model evaluation**

*1.1. Feature Generation*

Five drug-drug similarity measures and two disease-disease similarity measures were computed to generate features for the classifier. The drug-drug similarity is calculated using a set of data including chemical similarity, side effect similarity, and similarities based on target sequence and gene ontology annotations. The disease-disease similarity measure take into account the semantic similarity of disease phenotypes. All similarity scores between entities (drugs or diseases) are normalized in the range (0,1).

The drug similarity calculations are further described below:

**1- Chemical Based Similarity:**
Similarity between drugs based on molecular fingerprints were calculated using SMILES notations. The Open Drug Discovery Toolkit (ODDT) Python API [Wójcikowski] is used to generate chemical similarity scores. This tool converts the SMILES string of each drug into a fingerprint represented by a bit vector (166-bit for MACCS keys) and calculates a Jaccard\cite{jaccard1912distribution} score of the fingerprints for the similarity of two drugs. Jaccard score is the size of intersection over the union of fingerprint vectors and is calculated as follows:

$$Jaccard(X, Y) = \frac{|X \cap Y|}{|X \cup Y|}$$

X and Y represent the fingerprint vectors of two drugs.

**2- Side Effect Based Similarity:**
SIDER \cite{kuhn2015sider} is an online database of text mined drug indications and drug side effects. SIDER was automatically constructed by text mining of drug product labels and are known to contain false positives. Each drug might be associated with a set of side effects. Side effect based similarity between the two drugs was computed using the Jaccard score between their known side effects.

**3- Sequence Based Similarity:**
This similarity was computed from the Smith Waterman sequence alignment score of each of their targets. The alignment score is normalized by the procedure suggested by [Bleakley2019] which applies a normalization by dividing the alignment score by the geometric mean of the alignment scores between each sequence itself. For drug with more than one target gene, the average of each target's highest alignment scores were taken.

**4- Gene Ontology based Similarity:**
Gene Ontology (GO) based similarity scores were calculated according to Resnik's measure \cite{resnik1999semantic} using SML toolkit (SML 0.9) \cite{harispe2013semantic}. SML toolkit takes Gene Ontology (GO) and drug-related gene annotations as input and outputs drug-drug similarity scores.

**5- Protein-Protein Interaction Closeness:**

The distance between target proteins of the two drugs on the human protein-protein interaction network was translated to a similarity score. The score is then normalized between 0 and 1 as described by Perlman et al. \cite{perlman2011combining}. For drugs with more than one target, each target's highest similarity score was taken and averaged over the contribution of each target in a drug.

Two disease-disease similarity measures were calculated as follows:

**1- Similarity between OMIM diseases based on medical description of diseases (MeSH terms):**

This similarity is based on a text mining scheme described by \cite{van2006text}. After obtaining a list of MeSH terms for every OMIM disease description, we calculated a similarity score between each disease pair by taking cosine similarity measure of their MeSH terms.

**2- Similarity between OMIM diseases based on HPO terms:**

We collected Human Phenotype terms in each OMIM disease description and subsequently computed similarity between disease terms with Resnik's measure using SML toolkit with Human Phenotype Ontology (HPO) \cite{kohler2016human}.

The similarity measures were added to the feature matrix for classifier learning, prediction, and cross-validation. The feature matrix consists of a set of drug-disease scores, combining drug-drug and disease-disease similarity measures. Thus, we combine 5 drug-drug similarity measures and 2 disease-disease similarity measures, resulting in 10 features. For any drug-disease association **($d_r$ ,$d_i$),** the association score is calculated by comparing the query association to all known drug-disease associations **($d'_r$ ,$d'_i$)** as described by the following formula:

$$Score(d_r, d_i) = \max_{d'_r, d'_i \neq d_r, d_i} \sqrt{S(d_r, d'_r) \times (S(d_i, d'_i))}$$

where S($d_r$ ,$d'_r$) is the drug-drug similarity score between the drug in question ($d_r$) and drugs with known associations and S($d_i$ ,$d'_i$) is the disease-disease similarity score between the disease in question and diseases with known associations. Two similarity scores were combined by computing the weighted geometric mean. The final score for the query association is the maximum score of the combined scores for all known associations.

### *1.2. Performance Evaluation*

10 fold cross-validation scheme was used for evaluating the performance of the classifier. The PREDICT uses 2 different cross-validation approaches: One where 10 % of drugs is hidden and one where 10 % of associations is hidden. In the first strategy, we randomly remove 10% of all drugs in the gold standard and consequently remove all the known indications associated with them. The positive training set consists of the remaining 90% of drugs and the indications associated with them. The negative training set consists of randomly generated drug-disease associations not in the positive set and it is twice as large as the positive set. The positive test set includes the 10% of the drugs that were removed and the indications associated with them and the negative test set includes randomly generated drug-disease associations not in the positive test set. For the second approach, we divided

the known associations into 90% positive training and 10% positive test sets, while negative training and test sets were built using randomly generated drug-disease associations from respective sets.
