# Supplementary material for: Towards FAIR protocols and workflows: The OpenPREDICT case study
Source: arXiv:1911.09531 source file (2019-11-20)
Supplement: Supplementary file 3 [file cs-43016-Appendix_3__SPARQL_queries_for_competency_questions.pdf]

## Appendix 3: SPARQL queries for competency questions

http://graphdb.dumontierlab.com/sparql (choose *openpredict* repository)

The namespaces used are listed below:

"schema" : "http://schema.org#",
"bpmn" : "http://dkm.fbk.eu/index.php/BPMN2_Ontology#",
"edam" : "http://edamontology.org/",
"owl" : "http://www.w3.org/2002/07/owl#",
"reprod" : "https://w3id.org/reproduceme#",
"fabio" : "http://purl.org/spar/fabio/",
"xsd" : "http://www.w3.org/2001/XMLSchema#",
"opredict" : "http://purl.org/plex/Instances/OpenPREDICT#",
"pwo" : "http://purl.org/spar/pwo#",
"rdfs" : "http://www.w3.org/2000/01/rdf-schema#",
"p-plan" : "http://purl.org/net/p-plan#",
"rdf" : "http://www.w3.org/1999/02/22-rdf-syntax-ns#",
"mls" : "http://www.w3.org/ns/mls#",
"sh" : "http://www.w3.org/ns/shacl#",
"dul" : "http://www.ontologydesignpatterns.org/ont/dul/DUL.owl#",
"dcat" : "http://www.w3.org/ns/dcat#",
"prov" : "http://www.w3.org/ns/prov#",
"dc" : "http://purl.org/dc/terms/",
"opmw" : "http://www.opmw.org/ontology/"

***CQ1.1: Which steps are meant to be executed manually and which to be executed computationally?***

The SPARQL query that can be used for answering this question can be formulated as:

```
SELECT ?step ?stepType ?instructions ?description
WHERE
    {
        values ?stepType { bpmn:ManualTask bpmn:ScriptTask }

        ?instructions rdf:type p-plan:Plan.
        ?step rdf:type ?stepType.
        ?step dul:isDescribedBy ?instructions.

        ?instructions dc:description ?description.
        ?step p-plan:isStepOfPlan
opredict:Plan_Main_Protocol_v01.
    }
```

***CQ1.2: For the manual parts, who are the developers and who are the agents responsible to execute each step?***

The SPARQL query that can be used for answering this question can be formulated as:

```
SELECT ?step ?role ?agent ?creator ?publisher ?instructions ?description
WHERE
    {
        values ?stepType { bpmn:ManualTask }

        ?instructions rdf:type p-plan:Plan.
        ?step rdf:type ?stepType.
        ?step dul:isDescribedBy ?instructions.

        ?instructions dc:description ?description.
        ?association prov:hadPlan ?instructions.
        ?association prov:agent ?agent.
        ?association prov:hadRole ?role.
        OPTIONAL {?plan dc:creator ?creator}
        OPTIONAL {?plan dc:publisher ?publisher}

        ?step p-plan:isStepOfPlan
opredict:Plan_Main_Protocol_v01.
    }
```

***CQ1.3: Which datasets were used as input for the computational steps and their respective formats?***

The SPARQL query that can be used for answering this question can be formulated as:

```
SELECT ?step ?instructions ?usage ?usageEntity ?downloadURL ?dataFormat ?dataFormatLabel
WHERE
{
    ?usageEntity rdf:type dcat:Distribution.
    ?usage prov:entity ?usageEntity.
    ?plan prov:qualifiedUsage ?usage.
    ?step dul:isDescribedBy ?plan.
    ?step rdf:type edam:operation_2409.

    ?usageEntity dcat:mediaType ?dataFormat
    OPTIONAL { ?dataFormat rdfs:label ?dataFormatLabel.}

    OPTIONAL { ?usageEntity dcat:downloadURL ?downloadURL.}
    OPTIONAL { ?plan dc:description ?instructions.}
    OPTIONAL { ?step p-plan:hasInputVar ?varInput.}
    OPTIONAL { ?step p-plan:hasOutputVar ?varOutput.}

    ?step p-plan:isStepOfPlan opredict:Plan_Main_Protocol_v01.

}
```

***CQ1.4: What are the inputs and outputs of manual steps?***

The SPARQL query that can be used for answering this question can be formulated as:

```
SELECT ?step ?varInput ?varOutput ?instructions ?description
WHERE
    {
        values ?stepType { bpmn:ManualTask}

        ?instructions rdf:type p-plan:Plan.
        ?step dul:isDescribedBy ?instructions.

        ?instructions dc:description ?description.
        OPTIONAL { ?step p-plan:hasInputVar ?varInput.}
        OPTIONAL { ?step p-plan:hasOutputVar ?varOutput.}
        ?step                    p-plan:isStepOfPlan
opredict:Plan_Main_Protocol_v01.
    }
ORDER BY DESC(?varInput)
```

***CQ2.1: What are the main steps of OpenPREDICT protocol?***

The SPARQL query that can be used for answering this question can be formulated as:

```
SELECT ?stepA ?stepB
WHERE
{
    ?stepA p-plan:isStepOfPlan opredict:Plan_Main_Protocol_v01.
    ?stepA dul:precedes ?stepB.

    OPTIONAL {
            opredict:Plan_Main_Protocol_v01 pwo:hasFirstStep ?stepTopLevel.
            ?stepTopLevel dul:precedes ?stepB.
        }
}
ORDER BY  DESC(?stepTopLevel)
```

***CQ2.2: What are the steps of a plan and how each step instruction is described?***

The SPARQL query that can be used for answering this question can be formulated as:

```
SELECT ?language ?instructions ?description ?step
WHERE
{
    ?instructions rdf:type p-plan:Plan.
    ?step dul:isDescribedBy ?instructions.
    ?instructions dc:description ?description.
    ?instructions dc:language ?language.
```

```
}
```

***CQ2.3: What instructions specify the code used in OpenPREDICT steps?***

The SPARQL query that can be used for answering this question can be formulated as:

```
SELECT ?specInstruction ?specification ?instructions ?description ?step ?language
WHERE
{
    ?instructions rdf:type p-plan:Plan.
    ?step dul:isDescribedBy ?instructions.
    ?step rdf:type bpmn:ScriptTask.
    ?instructions dc:description ?description.
    ?instructions dc:language ?language.
    OPTIONAL
    {
        ?instructions dul:isDescribedBy ?specInstruction.
        ?specInstruction dc:description ?specification.
    }
}
ORDER BY ?step
```

***CQ3.1: What are the existing versions of a workflow and what are their provenance?***

The SPARQL query that can be used for answering this question can be formulated as:

```
SELECT ?workflow  ?wflVersion ?creator ?createDate
WHERE
{
    ?workflow rdf:type dul:Workflow.
    ?workflow dc:hasVersion ?wflVersion.
    ?workflow dc:creator ?creator.
    ?workflow dc:created ?createDate.
}
```

***CQ3.2: Which instructions were removed/changed/added from one version to another?***

***Removed from version 0.1 to version 0.2:***

The SPARQL query that can be used for answering this question can be formulated as:

```
SELECT *
WHERE
{
    ?step p-plan:isStepOfPlan opredict:Plan_Main_Protocol_v01.
    ?step dul:isDescribedBy ?instruction.
    ?step rdf:type ?stepType.
    values ?stepType { bpmn:ManualTask bpmn:ScriptTask }

    FILTER NOT EXISTS
    {
        ?step p-plan:isStepOfPlan opredict:Plan_Main_Protocol_v02.
```

```
    }

    FILTER NOT EXISTS
    {
        ?instructionNextVersion prov:wasRevisionOf ?instruction.
        ?stepNextVersion dul:isDescribedBy ?instructionNextVersion.
        ?stepNextVersion p-plan:isStepOfPlan opredict:Plan_Main_Protocol_v02.
    }

}
```

***Changed from version 0.1 to version 0.2:***

The SPARQL query that can be used for answering this question can be formulated as:

```
SELECT *
WHERE
{
    ?planNewVersion prov:wasRevisionOf ?planPriorVersion.
    ?planNewVersion dc:description ?planNewVersionDesc.
    ?planPriorVersion dc:description ?planPriorVersionDesc.
    FILTER (?planNewVersionDesc != ?planPriorVersionDesc).

}
```

***Added from version 0.1 to version 0.2:***

The SPARQL query that can be used for answering this question can be formulated as:

```
SELECT *
WHERE
{
    ?step p-plan:isStepOfPlan opredict:Plan_Main_Protocol_v02.
    ?step dul:isDescribedBy ?instruction.
    ?step rdf:type ?stepType.
    values ?stepType { bpmn:ManualTask bpmn:ScriptTask }

    FILTER NOT EXISTS
    {
        ?step p-plan:isStepOfPlan opredict:Plan_Main_Protocol_v01.
    }
    FILTER NOT EXISTS
    {
        ?instruction prov:wasRevisionOf ?instructionPriorVersion.
        ?stepPriorVersion dul:isDescribedBy ?instructionPriorVersion.
        ?stepPriorVersion p-plan:isStepOfPlan opredict:Plan_Main_Protocol_v01.
    }
}
```

***CQ3.3: Which steps were automatized from one version to another?***

The SPARQL query that can be used for answering this question can be formulated as:

```
SELECT ?stepPriorVersion ?planPriorVersion ?stepNewVersion ?planNewVersion
WHERE
{
	?planNewVersion prov:wasRevisionOf ?planPriorVersion.
	?planNewVersion dc:description ?planNewVersionDesc.
	?planPriorVersion dc:description ?planPriorVersionDesc.
	?stepNewVersion dul:isDescribedBy ?planNewVersion.
	?stepNewVersion rdf:type ?stepNewVersionType.
	?stepPriorVersion dul:isDescribedBy ?planPriorVersion.
	?stepPriorVersion rdf:type ?stepPriorVersionType.

	values ?stepPriorVersionType { bpmn:ManualTask}.
	values ?stepNewVersionType { bpmn:ScriptTask}

}
```

***CQ3.4: Which datasets were removed/changed/added for the different versions?***

The SPARQL query that can be used for answering this question can be formulated as:

This question can be answered by using the same query of CQ1.3 (datasets used), changing the filter to include v.0.2. Therefore, the instruction below should be removed:

```
?step p-plan:isStepOfPlan opredict:Plan_Main_Protocol_v01.
```

and replaced by:

```
OPTIONAL {?step p-plan:isStepOfPlan opredict:Plan_Main_Protocol_v01}
OPTIONAL {?step p-plan:isStepOfPlan opredict:Plan_Main_Protocol_v02}
```

```
SELECT ?step ?instructions ?usage ?usageEntity ?downloadURL ?dataFormat ?dataFormatLabel
WHERE
{
	?usageEntity rdf:type dcat:Distribution.
	?usage prov:entity ?usageEntity.
	?plan prov:qualifiedUsage ?usage.
	?step dul:isDescribedBy ?plan.
	?step rdf:type edam:operation_2409.

	?usageEntity dcat:mediaType ?dataFormat
	OPTIONAL { ?dataFormat rdfs:label ?dataFormatLabel.}

	OPTIONAL { ?usageEntity dcat:downloadURL ?downloadURL.}
	OPTIONAL { ?plan dc:description ?instructions.}
	OPTIONAL { ?step p-plan:hasInputVar ?varInput.}
	OPTIONAL { ?step p-plan:hasOutputVar ?varOutput.}
```

```
        OPTIONAL {?step p-plan:isStepOfPlan opredict:Plan_Main_Protocol_v01}
          OPTIONAL {?step p-plan:isStepOfPlan opredict:Plan_Main_Protocol_v02}

  }
```

***CQ3.5: Which workflow version was used in each execution and what was generated?***

The SPARQL query that can be used for answering this question can be formulated as:

```
SELECT ?plan ?version ?execution ?stepExecuted
WHERE
{
        ?execution rdf:type p-plan:Activity.
        ?execution p-plan:correspondsToStep ?stepExecuted.
        ?stepExecuted p-plan:isStepOfPlan ?plan.
        ?plan rdf:type dul:Workflow.
        ?plan dc:hasVersion ?version.
}
ORDER BY ?version
```

```
  SELECT ?plan ?version ?execution ?stepExecuted ?wflExecArtifact
  WHERE
  {
        ?execution rdf:type p-plan:Activity.
        ?execution p-plan:correspondsToStep ?stepExecuted.
        ?stepExecuted p-plan:isStepOfPlan ?plan.
        ?plan rdf:type dul:Workflow.
        ?plan dc:hasVersion ?version.
        ?execution prov:generated ?wflExecArtifact.
  }
  ORDER BY ?version
```
